# Supplementary material for: Mean Opinion Score as a New Metric for User-Evaluation of XAI Methods
Source: arXiv:2407.20427 source file (2024-07-29)
Supplement: Supplementary file 1 [file appendices.tex]

\chapter{Appendix A} 
Here you can present all the materials that help the understanding of your work, but either 1) not your work, 2) not necessary to understanding, 3) simply just interesting things not directly related to your topic, or 4) your text already exceeded 120 pages, and need to make it shorter by moving parts to appendix... Also, if you have a large number of images, code, or measurement data, it is required to insert them here rather than in chapters. You can have multiple appendices (possibly separated into multiple files) as it suits the content of the supplemental material.
